# Supplementary material for: The initial charge separation step in oxygenic photosynthesis
Source: arXiv:2107.11112 source file (2021-07-23)
Supplement: Supplementary file 1 [file SI.pdf]

Supplementary Information

# The initial charge separation step in oxygenic photosynthesis

*Yusuke Yoneda,[1,2,5] Eric A. Arsenault,[1,2,3] Kaydren Orcutt,[1] Masakazu Iwai[2,4] and Graham R. Fleming[1,2,3*]*

[1]*Department of Chemistry, University of California, Berkeley, CA 94720, USA*

[2]*Molecular Biophysics and Integrated Bioimaging Division, Lawrence Berkeley National Laboratory, Berkeley, CA 94720, USA*

[3]*Kavli Energy Nanoscience Institute at Berkeley, Berkeley, CA 94720, USA*

[4]*Department of Plant and Microbial Biology, University of California, Berkeley, CA 94720, USA*

[5]*Present Address: Research Center of Integrative Molecular Systems, Institute for Molecular Science, National Institute of Natural Sciences, Okazaki, Aichi, 444-8585, Japan*

[*]grfleming@lbl.gov

## Experimental Methods

**Two-dimensional electronic-vibrational spectroscopy.** A detailed description for the experimental setup of two-dimensional electronic-vibrational (2DEV) spectroscopy can be found elsewhere.[1] Briefly, the output of a Ti:sapphire oscillator (Vitara-S, Coherent) was regeneratively amplified with a 1 kHz repetition rate (Legend Elite, Coherent), an energy of 1 mJ/pulse and a pulse duration of 40 fs. The amplified pulse was divided into two and one was used to pump a home-built visible non-collinear optical parametric amplifier (NOPA). The other pulse was used to generate a mid-IR probe pulse (centered at 5.9 μm) by difference frequency generation with signal and idler pulses from a near-IR collinear OPA. The output of the NOPA (centered at 675 nm, 60 nm fwhm) was compressed to 20 fs at the sample position using a pair of prisms and an acousto-optic dispersive programmable filter (AODPF, Dazzler, Fastlite). The pulse pair was introduced to a retroreflector on a motorized translation stage to control the waiting time, $T$, between the pump and probe pulses. The total power of the pump pulses was set at 80 nJ and the pulses were focused into the sample with spot size of 250 μm. The mid-IR pulse was divided by a 50:50 beam splitter to form probe and reference beams. The probe and reference beams were dispersed by a spectrometer (Horiba, Triax 180) and detected by a 64-pixel HgCdTe dual array (Infrared Systems Development). The cross-correlation

between visible and mid-IR pulses was estimated to be 130 fs by a step-like transient IR response of a 50 μm Ge plate.

For each waiting time, a 2DEV spectrum was acquired by using the AODPF to scan the $t_1$ delay over 0-100 fs with 2.5 fs steps. For each $t_1$ delay, the signal was acquired with the relative phase between the pump pulses $\varphi_{12}$ set by 0, 2π/3 and 4π/3, and the desired signal was isolated by a 3×1×1 phase cycling scheme.[2,3] The excitation axis was obtained by a Fourier transformation over $t_1$. The signal was collected in the fully rotated frame with respect to $t_1$. For 2D-EADS analysis, the detection range was selected to be $\omega_{det.}$ = 1620-1740 $cm^{-1}$ because the dynamics in this range most fully reflects CS.

**Sample preparation.** All procedures for sample preparation were performed in the dark to minimize exposure to light as much as possible. We first isolated PSII-enriched membranes according to the previous literature with some modifications as follows.[4,5] We obtained spinach leaves (*Spinacia oleracea*) from a local store and kept in the dark overnight at 4 °C. The spinach leaves were briefly ground using a Waring blender in a buffer containing 50 mM MES-NaOH (pH 6.0), 400 mM NaCl, and 2 mM $MgCl_2$ at 4 °C. The ground tissues were filtered through 4 layers of Miracloth (Millipore), and the filtered homogenate was centrifuged at 1,400 × g for 10 min at 4 °C. The pellet was resuspended with a buffer containing 50 mM MES-NaOH (pH

6.0), 150 mM NaCl, and 5 mM $MgCl_2$, and resuspension was centrifuged at 4,000 × g for 10 min at 4 °C. The pellet was then resuspended with a buffer containing 50 mM MES-NaOH (pH 6.0), 15 mM NaCl, and 5 mM $MgCl_2$, and resuspension was centrifuged at 6,000 × g for 10 min at 4 °C. The pelleted thylakoid membranes were resuspended with the same buffer, and the concentration of chlorophylls was quantified by using 80% (v/v) acetone as described previously.[6] The thylakoid membranes (2.1 mg Chl/mL) were solubilized with 3.75% (w/v) Triton X-100 for 20 min on ice. The solution was centrifuged at 3,500 × g for 5 min at 4 °C. The supernatant was collected and further centrifuged at 40,000 × g for 30 min at 4 °C. The pelleted PSII-enriched membranes were washed with the same buffer and centrifuged again at 40,000 × g for 30 min at 4 °C. The PSII-enriched membranes were resuspended with a buffer containing 50 mM MES-NaOH (pH 6.0), 15 mM NaCl, 5 mM $MgCl_2$, and 400 mM sucrose, flash-frozen in liquid nitrogen, and stored at -80 °C until the following isolation procedures.

We isolated PSII-RC according to the previous literature with some modifications as follows.[7–9] The PSII-enriched membranes (1 mg Chl/mL) were solubilized with 4% (w/v) Triton X-100 in a buffer containing 50 mM Tris-HCl (pH 7.2) for 1 h on ice with gentle stirring. The solution was centrifuged at 33,000 × g for 1 h at 4 °C. The supernatant was collected and loaded onto an anion exchange column (Toyopearl DEAE-650S resin) which was equilibrated

with a buffer containing 50 mM Tris-HCl (pH 7.2), 30 mM NaCl, and 0.05% (w/v) Triton X-100 at 4 °C. The column was washed with the same buffer at a flow rate of 2.6 mL/min until the eluate showed the 417:435 nm ratio of about 1.16. Then, the column was subjected to a NaCl linear gradient from 30 to 200 mM at a flow rate of 1 mL/min. The green fraction eluted at 90-120 mM NaCl was collected. Then, polyethylene glycol 3350 was slowly added to the collected fraction at the final concentration of 0.325 g/mL, and the mixture was incubated for 30 min on ice with gentle stirring. The solution was centrifuged at 31,300 × g for 15 min at 4 °C. The pelleted PSII RC was resuspended with the buffer containing 50 mM Tris-HCl (pH 7.2), 0.4 M sucrose, 0.1% (w/v) n-dodecyl-β-D-maltoside (Anatrace) prepared with $D_2O$. The PSII-RC was flash-frozen and stored at -80 °C until 2DEV measurements.

For the spectroscopic experiments, the PSII-RC sample was mixed with glycerol-$d_8$ in a 80:20 (v/v) glycerol:PSII-RC ratio. The sample cell was constructed from two $CaF_2$ plates with a kapton spacer. The maximum optical density of the PSII-RC sample in the investigated visible range was set at ~1.0 with a path length of 200 μm. The sample was placed in an optical cryostat (OptistatDN2, Oxford Instruments) at 77 K.

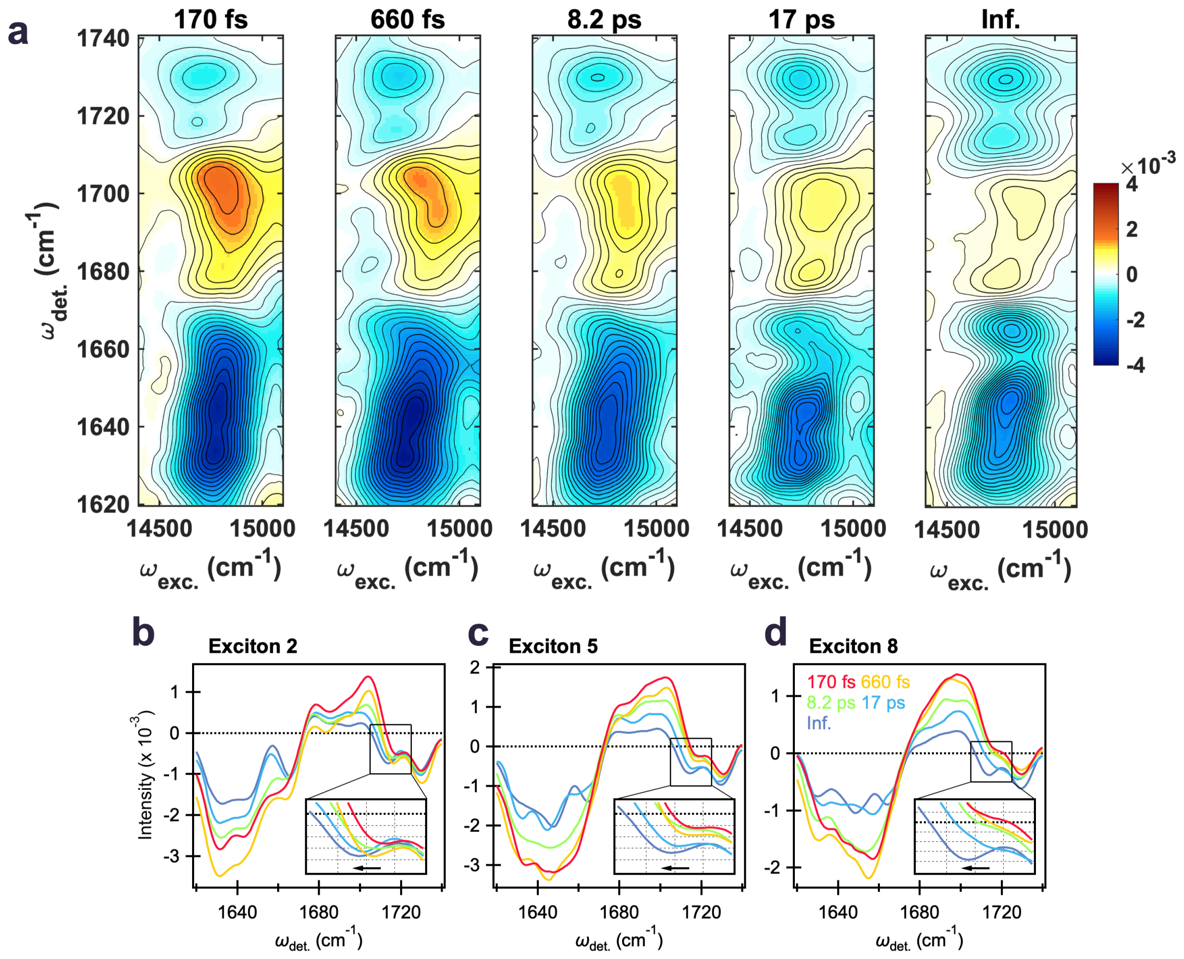


**Figure S1.** Two dimensional-evolution associated difference spectra (2D-EADS) of PSII-RC (a). Five components were required for a reasonable fit with time constants of 170 fs, 660 fs, 8.2 ps, 17 ps and a non-decaying offset component (longer than current detection time range of 100 ps). Each 2D-EADS evolves into the next one with the time constants listed above. Contour levels are drawn in 5% intervals. The time-dependent evolution of excitons 2, 5, and 8 are shown in (b)-(d), respectively.

## References

1. Oliver, T. A. A., Lewis, N. H. C. & Fleming, G. R. Correlating the motion of electrons and nuclei with two-dimensional electronic-vibrational spectroscopy. *Proc. Natl. Acad. Sci.* **111**, 10061–10066 (2014).

2. Zhang, Z., Wells, K. L., Hyland, E. W. J. & Tan, H. S. Phase-cycling schemes for pump-probe beam geometry two-dimensional electronic spectroscopy. *Chem. Phys. Lett.* **550**, 156–161 (2012).

3. Fleming, G. R., Lewis, N. H. C., Arsenault, E. A., Wu, E. C. & Oldemeyer, S. Two-Dimensional Electronic Vibrational Spectroscopy. in *Coherent Multidimensional Spectroscopy* (ed. Cho, M.) 35–49 (Springer Singapore, 2019). doi:10.1007/978-981-13-9753-0_2.

4. Berthold, D. A., Babcock, G. T. & Yocum, C. F. A highly resolved, oxygen-evolving photosystem II preparation from spinach thylakoid membranes. EPR and electron-transport properties. *FEBS Lett.* **134**, 231–234 (1981).

5. Caffarri, S., Kouřil, R., Kereïche, S., Boekema, E. J. & Croce, R. Functional architecture of higher plant photosystem II supercomplexes. *EMBO J.* **28**, 3052–3063 (2009).

6. Porra, R. J., Thompson, W. A. & Kriedemann, P. E. Determination of accurate extinction coefficients and simultaneous equations for assaying chlorophylls a and b extracted with four different solvents: verification of the concentration of chlorophyll standards by atomic absorption spectroscopy. *Biochim. Biophys. Acta - Bioenerg.* **975**, 384–394 (1989).

7. Nanba, O. & Satoh, K. Isolation of a photosystem II reaction center consisting of D-1 and D-2 polypeptides and cytochrome b-559. *Proc. Natl. Acad. Sci.* **84**, 109–112 (1987).

8. McTavish, H., Picorel, R. & Seibert, M. Stabilization of Isolated Photosystem II Reaction Center Complex in the Dark and in the Light Using Polyethylene Glycol and an Oxygen-Scrubbing System. *Plant Physiol.* **89**, 452–456 (1989).

9. Seibert, M. & Picorel, R. Isolation of Photosystem II Reaction Center Complexes from Plants. in *Photosynthesis Research Protocols* (ed. Carpentier, R.) 17–27 (Humana Press, 2011). doi:10.1007/978-1-60761-925-3_3.
